# Supplementary material for: SALA: Soft Assignment Local Aggregation for Parameter Efficient 3D Semantic Segmentation
Source: arXiv:2012.14929 source file (2021-04-05)
Supplement: Supplementary file 1 [file supmat.tex]

% % % This version of CVPR template is provided by Ming-Ming Cheng.
% % % Please leave an issue if you found a bug:
% % % https://github.com/MCG-NKU/CVPR_Template.

% \documentclass[review]{cvpr}
% %\documentclass[final]{cvpr}

% \usepackage{times}
% \usepackage{epsfig}
% \usepackage{graphicx}
% \usepackage{amsmath}
% \usepackage{amssymb}

% % Include other packages here, before hyperref.
% \newcommand{\SG}[1]{ {\color{red}[SG: #1]}}
% \newcommand{\BG}[1]{ {\color{red}[\textbf{BG}: \emph{#1}]}}
% \newcommand{\ali}[1]{ {\color{blue}[Ali: #1]}}

% % If you comment hyperref and then uncomment it, you should delete
% % egpaper.aux before re-running latex.  (Or just hit 'q' on the first latex
% % run, let it finish, and you should be clear).
% \usepackage[pagebackref=true,breaklinks=true,colorlinks,bookmarks=false]{hyperref}


% \def\cvprPaperID{1275} % *** Enter the CVPR Paper ID here
% \def\confYear{CVPR 2021}
% %\setcounter{page}{4321} % For final version only


% \begin{document}
% \appendix
% \onecolumn

% %%%%%%%%% TITLE
% \title{Supplementary Material For: \\SALA: Soft Assignment Local Aggregation for 3D Semantic Segmentation}

% \author{First Author\\
% Institution1\\
% Institution1 address\\
% {\tt\small firstauthor@i1.org}
% % For a paper whose authors are all at the same institution,
% % omit the following lines up until the closing ``}''.
% % Additional authors and addresses can be added with ``\and'',
% % just like the second author.
% % To save space, use either the email address or home page, not both
% \and
% Second Author\\
% Institution2\\
% First line of institution2 address\\
% {\tt\small secondauthor@i2.org}
% }
% \maketitle

% \section{Architecture Blocks}

% \begin{figure*}[htb]
%     \centering
%     \includegraphics[trim = 30mm 30mm 30mm 5mm, clip, width=\linewidth]{supplementary/suparchitecture.pdf}
%     \caption{\textbf{Architecture.} Unified architecture framework from \cite{closerlook3d}.
%     % The architecture used in the unified framework proposed in \cite{closerlook3d}. %The architecture details were initially introduced in \cite{kpconv}. 
%     Both Residual and Strided Residual Blocks have local aggregation functions within. The strided residual blocks acts as a pooling operator in which point cloud resolution is reduced using grid-subsampling. The grid size is doubled going deeper in the encoder. %$N$ refers to the input point cloud resolution. 
%     $C$ refers to channel output of first encoding layer. $\gamma=2$ is the residual bottlneck ratio. $r$ refers to the encoder point cloud downsampling ratio.}
%     \label{fig:archblocks}
%     \vspace{-2mm}
% \end{figure*}

% \section{Training and Inference Settings}
% We evaluate Soft Assignment Local Aggregation (SALA) function in the unified framework proposed in \cite{closerlook3d}. This includes data pre-processing, augmentation, architecture (see Figure \ref{fig:archblocks}), and training and inference schemes. Models are trained with cross-entropy loss and $L_2$ regularizer on learned weights.

% \subsection{S3DIS}
% The initial inputs to the model are lifted ZRGB1 features ($d_0=5$). Following \cite{closerlook3d,kpconv}, the data is augmented with random rotations along the z-axis, random scaling (ratios 0.7 to 1.3), random color drop, and additive Gaussian point perturbations with standard deviation $\delta=0.001$. The reported mIoU is a result of voting scheme employed in \cite{closerlook3d,kpconv}. A point cloud is divided using regular overlapping spheres. The logits of a point seen in different spheres are then averaged before Softmax and label assignment.

% \subsection{ScanNet}
% The initial inputs to the model are lifted RGB1 features ($d_0=4$). Following \cite{kpconv}, the data is augmented with random rotations along the z-axis, random scaling (ratios 0.9 to 1.1), random color drop, and additive Gaussian point perturbations with standard deviation $\delta=0.001$. The reported mIoU is as reported on ScanNet benchmarks website. Predictions on the test-set are collected using the same voting scheme discussed previously as in \cite{kpconv}.

% \subsection{PartNet}
% The initial inputs to the model are lifted XYZ1 features ($d_0=4$). Following \cite{closerlook3d}, the data is augmented with random scaling (ratios 0.8 to 1.2), and additive Gaussian point perturbations with standard deviation $\delta=0.001$. The reported mIoU is a result of voting scheme where logits are averaged over prediction on augmented test-set as in \cite{closerlook3d}. 

% \section{Quantitative and Qualitative Results}
% \subsection{S3DIS}
% Tables \ref{table:sups3disa5} and \ref{table:sups3dis6fold} show the per class IoU on S3DIS Area 5 and 6-fold-cross-validation benchmarks respectively. On both benchmarks, SALANet with $S=2$ groups achieves state-of-the-art (SOTA) performance. Sample qualitative results are showcased in Figure \ref{fig:supquals3dis}.

% \subsection{ScanNet}
% Table \ref{table:supscannet} shows the per class IoU on ScanNet test-set. SALANet with $S=2$ groups achieves competitive performance while using much less parameters in comparison with other SOTA methods with much more complex kernels. Sample qualitative results on validation-set are showcased in Figure \ref{fig:supqualscannet}.

% \subsection{PartNet}
% Table \ref{table:suppartnet} shows the per shape category mean part IoU (mpIoU) on PartNet test-set. \cite{closerlook3d} noted that increasing the output channel dimension $C$ is especially important on complex datasets such as PartNet. We vary the output channel dimension $C$ to test our model at different model learning capacities. Increasing the channel dimension compromises the efficiency of SALANet and does not consistently yield an improvement on the general performance.  This could be a result of potential overfitting. Yet, SALANet with $S=2$ groups achieves competitive performance in comparison with much larger models. Sample qualitative results on test-set are showcased in Figure \ref{fig:supqualpartnet}.

% \input{supplementary/s3disa5perclass}
% \input{supplementary/s3dis6foldperclass}
% \input{supplementary/supscannet}
% \clearpage

% \begin{figure*}[htb]
%     \centering
%     \includegraphics[trim = 2mm 35mm 2mm 30mm, clip, width=\linewidth]{supplementary/s3dis1.pdf}
%     \includegraphics[trim = 2mm 30mm 2mm 21mm, clip, width=\linewidth]{supplementary/s3dis2.pdf}
%     \caption{\textbf{Qualitative Results on S3DIS.} Sample qualitative results of SALANet with $S=2$ groups on S3DIS Area 5.}
%     \label{fig:supquals3dis}
%     \vspace{-2mm}
% \end{figure*}
% \clearpage

% \begin{figure*}[htb]
%     \centering
%     \includegraphics[trim = 2mm 5mm 2mm 5mm, clip, width=\linewidth]{supplementary/scannet1.pdf}
%     \includegraphics[trim = 2mm 5mm 2mm 5mm, clip, width=\linewidth]{supplementary/scannet2.pdf}
%     \includegraphics[trim = 10mm 90mm 10mm 90mm, clip, width=\linewidth]{supplementary/scannet3.pdf}
%     \caption{\textbf{Qualitative Results on ScanNet.} Sample qualitative results of SALANet with $S=2$ groups on ScanNet validation-set.}
%     \label{fig:supqualscannet}
%     \vspace{-2mm}
% \end{figure*}
% \clearpage
% \input{supplementary/partnetperclass}
% \begin{figure*}[htb]
%     \centering
%     \includegraphics[trim = 2mm 5mm 2mm 5mm, clip, width=\linewidth]{supplementary/partnet1.pdf}
%     \caption{\textbf{Qualitative Results on PartNet.} Sample qualitative results of SALANet with $S=2$ groups on PartNet test-set using output channel dimension $C=36$ and $C=72$}
%     \label{fig:supqualpartnet}
%     \vspace{-2mm}
% \end{figure*}
% \clearpage
% {\small
% \bibliographystyle{ieee_fullname}
% \bibliography{egbib}
% }

% \end{document}
